# Supplementary material for: Empowering News Recommendation with Pre-trained Language Models
Source: arXiv:2104.07413 source file (2021-04-15)
Supplement: Supplementary file 1 [file supplement.tex]

\section{Supplementary Materials}
